# Supplementary material for: Fair Contextual Multi-Armed Bandits: Theory and Experiments
Source: arXiv:1912.08055 source file (2019-12-13)
Supplement: Supplementary file 1 [file appendix.tex]

\onecolumn
\subsection*{Proof of Theorem~\ref{theo: unkown context}}
Let's define each block k as $B_k$ for convenience. \\
\textbf{First we analyze the total number of violations: }\\
For each $k$, by Hoeffding inequality and the union bound, we get that with a high probability at least $1 - \frac{M}{T^2}$, 
\begin{align*}
    \norm{q - \Bar{q}^k}_{\infty} \leq 2\sqrt{\frac{\log T}{\tau_k - 1}}
\end{align*}
Therefore, according to the definition of $\hat{\Omega}_q^k$, the above inequality implies that $q \in \hat{\Omega}_q^k$ with probability $1-\frac{M}{T^2}$. Then according to the definition of $\hat{\Omega}_P^k$, any $P_t$ inside $B_k$ will not violate the rate constraints, as long as $q \in \hat{\Omega}_q^k$. Therefore,
\begin{align*}
    \sum_{t=1}^T \E[\one\{P_t \notin \Omega\}] 
    =\sum_{t=1}^T \Pr{(P_t \notin \Omega)}
    = \sum_{k=1}^{\log T} \sum_{t \in B_k} \frac{M}{T^2} = \order(1) 
\end{align*}
\\
\textbf{Next analyze the regret bounds: }\\
Denote
\begin{align*}
    &P_* = \argmax_{P_* \in \Omega} \E \left[ \sum_{t=1}^T \inner{p_t^{j_t}-p_*^{j_t},l_t}\right],
    &P_*^k = \argmax_{P_* \in \hat{\Omega}_P^k} \E \left[ \sum_{t \in B_k} \inner{p_t^{j_t}-p_*^{j_t},l_t}\right]
\end{align*}
Then we can decompose the regret inside one block $B_k$ as 
\begin{align*}
    Reg_{B_k} = \E \left[ \sum_{t \in B_k} \inner{p_t^{j_t}-p_*^{j_t},l_t}\right]
    = \E \left[ \sum_{t \in B_k} \inner{p_t^{j_t}-p_*^{k,j_t},l_t}\right] + \E \left[ \sum_{t \in B_k} \inner{p_t^{k,j_t}-p_*^{j_t},l_t}\right]
\end{align*}
The first term can be bounded by $\order(\sqrt{KM|B_k|\log K})$ using the same FTRL proof as before.\\
Then we bound the second term. By the previous analysis in the number of violation, we know that with high probability $q \in \hat{\Omega}_q^k$. And thus $\norm{\hat{q} - q}_\infty \leq 4\sqrt{\frac{\log T}{\tau_k - 1}}, \forall \hat{q} \in \hat{\Omega}_q^k$. Therefore by applying Lemma~\ref{lem: unkown context}, we get 
\begin{align*}
     \E \left[ \sum_{t \in B_k} \inner{p_t^{t,j_t}-p_*^{j_t},l_t}\right] 
     &\leq  \sum_{t \in B_k} \sum_{i=1}^K \order(\frac{M}{u}\sqrt{\frac{\log T}{\tau_k - 1}}) l_t(i)\\
     &\leq \sum_{t \in B_k} \order(\frac{MK}{u}\sqrt{\frac{\log T}{\tau_k - 1}}) = \order(\frac{MK}{u}\sqrt{\log T |B_k|})
\end{align*}
Finally add up all the regret inside block we get 
\begin{align*}
    \sum_{k=1}^{\log T} Reg_{B_k}
    &= \sum_{k=1}^{\log T}\order(\sqrt{KM|B_k|\log K}) + \sum_{k=1}^{\log T}\order(\frac{MK}{u}\sqrt{\log T |B_k|})\\
    &\leq \order(\frac{MK}{u}\log T\sqrt{T}) \quad \text{ (By Cauchy–Schwarz) }
\end{align*}

\begin{lemma}
\label{lem: unkown context}
Suppose we have the distribution over context $\{ q\in \Delta_M | q(j) > u, \forall j \}$, and some time interval $\Gamma$. Define
\begin{align*}
    &\Omega_1(q_1) = \left\{ P=(p^1,p^2,\ldots,p^M)| p^1,\ldots,p^M \in \Delta_K \text{ and }  \sum_{j=1}^M q_1(j)p^j(i) \geq v, \forall i\in[K]\right\}\\
    &\Omega_2(q_1,\epsilon) = \bigcap_{q': \substack{\norm{q_1 - q'}_\infty} \leq \epsilon} \Omega_1(q')
\end{align*}
Then we will get
\begin{align*}
    \norm{\left[\argmin_{P_* \in \Omega_2(q_1,\epsilon)} \sum_{t \in \Gamma} \inner{p_*^{j_t},l_t} - \argmin_{P_* \in \Omega_1(q_1)} \sum_{t \in \Gamma} \inner{p_*^{j_t},l_t} \right]^j}_{\infty} \leq \order(\frac{M\epsilon}{u}), \forall j \in [M]
\end{align*}
This lemma guarantees that if we can estimate context distribution accurately, then the best collections of action distributions based on our estimation will also be close to the ground truth best collections of action distributions.
\end{lemma}

\begin{proof}
Let $P_1 = \argmin_{P_* \in \Omega_1(q_1)} \sum_{t \in \Gamma} \inner{p_*^{j_t},l_t}, P_2 = \argmin_{P_* \in \Omega_2(q_1,\epsilon)}\sum_{t \in \Gamma} \inner{p_*^{j_t},l_t}$ and $P_1 \neq P_2$. Then there must be at least one $i$ that, for some $\{ \epsilon'\in [-\epsilon,\epsilon]^M | \text{ and } \sum_{j=1}^M \epsilon'(j) = 0\}$, the following inequality holds
\begin{align*}
    \sum_{j=1}^M (q_1(j) - \epsilon'(j)) p_1^j(i) \geq  v - M\epsilon
\end{align*}
Easy to see that there always exists some $\xi^j$ that whose $\norm{\xi^j}_\infty \leq \frac{M\epsilon}{u}$ satisfying 
\begin{align*}
    \sum_{j=1}^M (q_1(j) - \epsilon'(j)) (p_1^j(i) + \xi^j(i)) \geq  v
\end{align*}
which means $p_1^j(i) + \xi^j(i) \in \Omega_2(q_1,\epsilon)$.
On the other hand, because $\Omega_2(q_1,\epsilon) \subseteq \Omega_1(q_1)$, so we can regard $P_2$ as a projection of $P_1$ on $\Omega_2(q_1,\epsilon)$, therefore for any 
\begin{align*}
    \norm{p_1^j - p_2^j}_\infty = \min_{\tilde{P} \in \Omega_2(q_1,\epsilon)} \norm{p_1^j - \tilde{p}_2^{j}}_\infty \leq \frac{M\epsilon}{u}
\end{align*}

\end{proof}
